# Supplementary material for: GarVerseLOD: High-Fidelity 3D Garment Reconstruction from a Single In-the-Wild Image using a Dataset with Levels of Details
Source: arXiv:2411.03047 source file (2024-11-05)
Supplement: Supplementary file 1 [file table_three_database.tex]

% \begin{table}[htbp]
%     \renewcommand{\arraystretch}{0.8}
%     \centering
%     \resizebox{0.4\textwidth}{!}{
%         \begin{tabular}{l|c|c|c|c|c}
%         % \hline 
%         \toprule
%         Category & Dress & Coat & Skirt & Top & Pant \\
%         \midrule
%         Garment Style Database & 863 & 760 & 538 & 350 & 358 \\
%         \midrule
%         Local Detail Database & 86 & 62 & 55 & 38 & 36 \\
%         \midrule
%         Garment Deformation Database & 622 & 605 & 456 & 582 & 589 \\
%         \midrule
%         Total & 1,571 & 1,427 & 1,049 & 970 & 983 \\
%         \bottomrule
%         \end{tabular}
%     }
%     \caption{Data statistics for each basic database.}
%     \label{tab:dataset}
% \end{table}
